# Supplementary material for: The junChS and junChS-F12 models: parameter-free efficient yet accurate composite schemes for energies and structures of non-covalent complexes
Source: arXiv:2110.03075 source file (2021-10-06)
Supplement: Supplementary file 1 [file SI.pdf]

# Supporting Information

## The junChS and junChS-F12 models: parameter-free efficient yet accurate composite schemes for energies and structures of non-covalent complexes


Jacopo Lupi,[†,¶] Silvia Alessandrini,[†,‡,¶] Cristina Puzzarini,[*,‡] and Vincenzo Barone[*,†]

†*Scuola Normale Superiore, Piazza dei Cavalieri 7, I-56126 Pisa, Italy*

‡*Dipartimento di Chimica "Giacomo Ciamician", Università di Bologna, Via F. Selmi 2, I-40126 Bologna, Italy.*

¶*J.L and S.A. contributed equally to this work.*

E-mail: cristina.puzzarini@unibo.it; vincenzo.barone@sns.it

Table S1: junChS-F12 NCP-energies (kJ·mol$^{-1}$): the various contributions for the A14 complexes.

| | "ref" | CC/junTZ | $\Delta$MP2$^{\infty}$/jun(T,Q)Z | MP2-CV/wCVTZ | Total | Rel. Error (%) | Abs. Error |
|---|---|---|---|---|---|---|---|
| $H_2O\cdots H_2O$ | -21.0832 | -21.4317 | 0.4631 | -0.1384 | -21.1070 | 0.11 | -0.02 |
| $NH_3\cdots NH_3$ | -13.2131 | -13.2529 | 0.1188 | -0.0605 | -13.1946 | -0.14 | 0.02 |
| HF···HF | -19.2213 | -19.6172 | 0.3155 | -0.1038 | -19.4055 | 0.96 | -0.18 |
| $CH_2O\cdots CH_2O$ | -18.9284 | -19.1210 | 0.0745 | -0.0506 | -19.0971 | 0.89 | -0.17 |
| HCN···HCN | -19.9828 | -20.1677 | 0.3029 | -0.1230 | -19.9878 | 0.02 | 0.00 |
| $C_2H_4\cdots C_2H_4$ | -4.6024 | -4.5937 | -0.0544 | -0.0482 | -4.6962 | 2.04 | -0.09 |
| $CH_4\cdots CH_4$ | -2.23007 | -2.1810 | 0.0298 | -0.0086 | -2.1598 | -3.15 | 0.07 |
| $H_2O\cdots NH_3$ | -27.3759 | -27.7949 | 0.4503 | -0.1766 | -27.5212 | 0.53 | -0.15 |
| $H_2O\cdots C_2H_4$ | -10.7696 | -10.8837 | 0.1783 | -0.0994 | -10.8049 | 0.33 | -0.04 |
| $C_2H_4\cdots CH_2O$ | -6.79482 | -6.8380 | -0.0105 | -0.0577 | -6.9061 | 1.64 | -0.11 |
| $NH_3\cdots C_2H_4$ | -5.78647 | -5.8409 | 0.0541 | -0.0532 | -5.8399 | 0.92 | -0.05 |
| $HF\cdots CH_4$ | -6.91615 | -7.1018 | 0.1460 | -0.0992 | -7.0550 | 2.01 | -0.14 |
| $H_2O\cdots CH_4$ | -2.8242 | -2.8971 | 0.1713 | -0.0261 | -2.7518 | -2.56 | 0.07 |
| $NH_3\cdots CH_4$ | -3.2175 | -3.3536 | 0.1629 | -0.0279 | -3.2186 | 0.03 | -0.001 |
| MAE | | | | | | 0.26 | -0.06 |

Table S2: jun-$(d,f)$H_ChS-F12 NCP-energies (kJ mol$^{-1}$): the various contributions for the A14 complexes.

| | "ref" | CC/junTZ-$d$H | $\Delta$MP2$^{\infty}$/jun(T,Q)Z-$d$H | MP2-CV/wCVTZ | Total | Rel. Error (%) | Abs. Error |
|---|---|---|---|---|---|---|---|
| $H_2O\cdots H_2O$ | -21.0832 | -21.4194 | 0.4617 | -0.1384 | -21.0961 | 0.06 | 0.01 |
| $NH_3\cdots NH_3$ | -13.2131 | -13.2161 | 0.0941 | -0.0605 | -13.1826 | 0.23 | -0.03 |
| HF···HF | -19.2213 | -19.5602 | 0.2534 | -0.1038 | -19.4105 | 0.98 | 0.19 |
| HCN···HCN | -19.9828 | -20.1691 | 0.3200 | -0.1230 | -19.9721 | 0.05 | -0.01 |
| $CH_4\cdots CH_4$ | -2.2301 | -2.1747 | 0.0325 | -0.0086 | -2.1508 | 3.56 | -0.08 |
| $CH_2O\cdots CH_2O$ | -18.9284 | -19.0957 | 0.0899 | -0.0506 | -19.0563 | 0.68 | 0.13 |
| $C_2H_4\cdots C_2H_4$ | -4.6024 | -4.5783 | -0.0628 | -0.0482 | -4.6893 | 1.89 | 0.09 |
| $H_2O\cdots C_2H_4$ | -10.7696 | -10.8734 | 0.1665 | -0.0993 | -10.8062 | 0.34 | 0.04 |
| $H_2O\cdots CH_4$ | -2.8242 | -2.8937 | 0.1691 | -0.0265 | -2.7512 | 2.59 | -0.07 |
| $H_2O\cdots NH_3$ | -27.3759 | -27.7545 | 0.4001 | -0.1765 | -27.5309 | 0.57 | 0.16 |
| $NH_3\cdots CH_4$ | -3.2175 | -3.3580 | 0.1714 | -0.0274 | -3.2140 | 0.11 | 0.00 |
| $NH_3\cdots C_2H_4$ | -5.7865 | -5.8372 | 0.0511 | -0.0530 | -5.8391 | 0.91 | 0.05 |
| $HF\cdots CH_4$ | -6.9162 | -7.0291 | 0.0898 | -0.0992 | -7.0386 | 1.77 | 0.12 |
| $C_2H_4\cdots CH_2O$ | -6.7948 | -6.8289 | 0.0016 | -0.0567 | -6.8840 | 1.31 | 0.09 |
| MAE | | | | | | 1.08 | 0.05 |

Table S3: junCBS+CV-F12 NCP-energies (kJ·mol$^{-1}$): the various contributions for the A14 complexes.

| | "ref" | CC-CBS/jun(T,Q)Z | CC-CV/wCVTZ | Total | Rel. Error (%) | Abs. Error |
|---|---|---|---|---|---|---|
| $H_2O \cdots H_2O$ | -21.0832 | -21.1486 | -0.1024 | -21.2510 | 0.80 | -0.17 |
| $NH_3 \cdots NH_3$ | -13.2131 | -13.2052 | -0.0397 | -13.2449 | 0.24 | -0.03 |
| HF···HF | -19.2213 | -19.4387 | -0.0678 | -19.5065 | 1.48 | -0.29 |
| $CH_2O \cdots CH_2O$ | -18.9284 | -19.0591 | 0.0476 | -19.0116 | 0.44 | -0.08 |
| HCN···HCN | -19.9828 | -19.8982 | -0.1201 | -20.0183 | 0.18 | -0.04 |
| $C_2H_4 \cdots C_2H_4$ | -4.6024 | -4.6129 | -0.0007 | -4.6136 | 0.24 | -0.01 |
| $CH_4 \cdots CH_4$ | -2.2301 | -2.1778 | 0.0015 | -2.1763 | -2.41 | 0.05 |
| $H_2O \cdots NH_3$ | -27.3759 | -27.5016 | -0.1367 | -27.6383 | 0.96 | -0.26 |
| $H_2O \cdots C_2H_4$ | -10.7696 | -10.7484 | -0.0378 | -10.7862 | 0.15 | -0.02 |
| $C_2H_4 \cdots CH_2O$ | -6.7948 | -6.8230 | 0.0001 | -6.8228 | 0.41 | -0.03 |
| $NH_3 \cdots C_2H_4$ | -5.7865 | -5.8003 | -0.0143 | -5.8146 | 0.49 | -0.03 |
| $HF \cdots CH_4$ | -6.9162 | -7.0312 | -0.0614 | -7.0926 | 2.55 | -0.18 |
| $H_2O \cdots CH_4$ | -2.8242 | -2.7652 | -0.0135 | -2.7787 | -1.61 | 0.05 |
| $NH_3 \cdots CH_4$ | -3.2175 | -3.2335 | -0.0116 | -3.2451 | 0.86 | -0.03 |
| MAE | | | | | 0.92 | 0.09 |

Table S4: junChS CP-energies (kJ·mol$^{-1}$): the various contributions for the A14 complexes.

| | "ref" | CC/junTZ | $\Delta$MP2$^{\infty}$/jun(T,Q)Z | MP2-CV/wCVTZ | Total | Rel. Error (%) | Abs. Error |
|---|---|---|---|---|---|---|---|
| $H_2O \cdots H_2O$ | -21.0832 | -19.3953 | -1.5582 | -0.1461 | -21.0996 | 0.08 | -0.02 |
| $NH_3 \cdots NH_3$ | -13.2131 | -11.8951 | -1.3311 | -0.0784 | -13.3046 | 0.69 | -0.09 |
| HF···HF | -19.2213 | -17.5377 | -1.8012 | -0.1118 | -19.4507 | 1.19 | -0.23 |
| $CH_2O \cdots CH_2O$ | -18.9284 | -16.2045 | -2.9410 | -0.0850 | -19.2305 | 1.60 | -0.30 |
| HCN···HCN | -19.9828 | -18.7592 | -1.0467 | -0.0700 | -19.8759 | -0.54 | 0.11 |
| $C_2H_4 \cdots C_2H_4$ | -4.6024 | -3.7738 | -0.9277 | -0.0484 | -4.7499 | 3.20 | -0.15 |
| $CH_4 \cdots CH_4$ | -2.2301 | -1.6577 | -0.5897 | -0.0064 | -2.2538 | 1.06 | -0.02 |
| $H_2O \cdots NH_3$ | -27.3759 | -25.4086 | -1.9709 | -0.1872 | -27.5667 | 0.70 | -0.19 |
| $H_2O \cdots C_2H_4$ | -10.7696 | -9.4665 | -1.2918 | -0.1003 | -10.8586 | 0.83 | -0.09 |
| $C_2H_4 \cdots CH_2O$ | -6.7948 | -5.7002 | -1.1790 | -0.0636 | -6.9427 | 2.18 | -0.15 |
| $NH_3 \cdots C_2H_4$ | -5.7865 | -4.9559 | -0.8829 | -0.0556 | -5.8943 | 1.86 | -0.11 |
| $HF \cdots CH_4$ | -6.9162 | -5.9096 | -1.1172 | -0.1006 | -7.1274 | 3.05 | -0.21 |
| $H_2O \cdots CH_4$ | -2.8242 | -2.3175 | -0.4339 | -0.0319 | -2.7833 | -1.45 | 0.04 |
| $NH_3 \cdots CH_4$ | -3.2175 | -2.6927 | -0.5117 | -0.0399 | -3.2443 | 0.83 | -0.03 |
| MAE | | | | | | 1.38 | 0.12 |

Table S5: junChS NCP-energies (kJ·mol$^{-1}$): the various contributions for the A14 complexes.

| | "ref" | CC/junTZ | $\Delta$MP2$^{\infty}$/jun(T,Q)Z | MP2-CV/wCVTZ | Total | Rel. Error (%) | Abs. Error |
|---|---|---|---|---|---|---|---|
| $H_2O \cdots H_2O$ | -21.0832 | -21.0233 | -0.2079 | -0.1429 | -21.3741 | 1.38 | -0.29 |
| $NH_3 \cdots NH_3$ | -13.2131 | -12.7819 | -0.4828 | -0.0784 | -13.3432 | 0.98 | -0.13 |
| HF$\cdots$HF | -19.2213 | -19.3800 | -0.0959 | -0.1140 | -19.5899 | 1.92 | -0.37 |
| $CH_2O \cdots CH_2O$ | -18.9284 | -18.2645 | -1.1814 | 0.0140 | -19.4319 | 2.66 | -0.50 |
| HCN$\cdots$HCN | -19.9828 | -20.5372 | 0.9151 | -0.0829 | -19.7049 | 1.39 | 0.28 |
| $C_2H_4 \cdots C_2H_4$ | -4.6024 | -4.7291 | -0.0019 | -0.0502 | -4.7813 | 3.89 | -0.18 |
| $CH_4 \cdots CH_4$ | -2.2301 | -2.0900 | -0.1193 | -0.0084 | -2.2176 | 0.56 | 0.01 |
| $H_2O \cdots NH_3$ | -27.3759 | -27.2308 | -0.2795 | -0.1782 | -27.6885 | 1.14 | -0.31 |
| $H_2O \cdots C_2H_4$ | -10.7696 | -10.7880 | -0.1205 | -0.1008 | -11.0094 | 2.23 | -0.24 |
| $C_2H_4 \cdots CH_2O$ | -6.7948 | -6.8647 | -0.1498 | -0.0587 | -7.0732 | 4.10 | -0.28 |
| $NH_3 \cdots C_2H_4$ | -5.7865 | -5.8092 | -0.1219 | -0.0556 | -5.9867 | 3.46 | -0.20 |
| $HF \cdots CH_4$ | -6.9162 | -7.0660 | 0.0317 | -0.1056 | -7.1399 | 3.23 | -0.22 |
| $H_2O \cdots CH_4$ | -2.8242 | -2.8609 | 0.1007 | -0.0297 | -2.7900 | 1.21 | 0.03 |
| $NH_3 \cdots CH_4$ | -3.2175 | -3.2828 | 0.0736 | -0.0297 | -3.2388 | 0.66 | -0.02 |
| MAE | | | | | | 2.06 | 0.22 |

Table S6: Geometries of the A14 complexes at different levels of theory. The inter-molecular parameters are highlighted in bold.

| | | CC/junVTZ | CC-F12/junTZ | CC-F12/junTZ+ MP2-CV(wCVTZ) | ChS | ChS+aug$\Delta\alpha$ | ChS+jun$\Delta\alpha$ | junChS | junCBS+CV-F12 | junChS-F12 | revDSD | Hobza |
|---|---|---|---|---|---|---|---|---|---|---|---|---|
| HCN···HCN | $r$(H1-C2) | 1.0688 | 1.0675 | 1.0664 | 1.0658 | 1.0663 | 1.0667 | 1.0656 | 1.0659 | 1.0658 | 1.0682 | 1.0687 |
| | $r$(C2-N3) | 1.1586 | 1.1553 | 1.1525 | 1.1504 | 1.1506 | 1.1506 | 1.1505 | 1.1508 | 1.1501 | 1.1556 | 1.1550 |
| | $r$(N3-H4) | 2.2167 | 2.2143 | 2.2114 | 2.2149 | 2.2059 | 2.2167 | 2.2164 | 2.2146 | 2.2162 | 2.2015 | 2.2253 |
| | $r$(**H4-C5**) | 1.0740 | 1.0729 | 1.0718 | 1.0718 | 1.0719 | 1.0729 | 1.0714 | 1.0717 | 1.0716 | 1.0740 | 1.0743 |
| | $r$(C5-N6) | 1.1609 | 1.1576 | 1.1548 | 1.1526 | 1.1529 | 1.1531 | 1.1528 | 1.1529 | 1.1522 | 1.1580 | 1.1572 |
| HF···HF | $r$(H1-F2) | 0.9231 | 0.9217 | 0.9212 | 0.9181 | 0.9211 | 0.9204 | 0.9179 | 0.9187 | 0.9184 | 0.9240 | 0.9199 |
| | $r$(**F2-H3**) | 1.8304 | 1.8280 | 1.8257 | 1.8244 | 1.8419 | 1.8468 | 1.8176 | 1.8212 | 1.8225 | 1.8261 | 1.8327 |
| | $r$(H3-F4) | 0.9257 | 0.9244 | 0.9239 | 0.9209 | 0.9249 | 0.9240 | 0.9208 | 0.9216 | 0.9213 | 0.9273 | 0.9227 |
| | $\theta$(**H3-F2-F1**) | 115.18 | 114.70 | 115.05 | 115.68 | 120.32 | 121.17 | 114.79 | 115.16 | 115.10 | 114.03 | 115.02 |
| | $\theta$(**F4-H3-F2**) | 170.63 | 169.41 | 169.67 | 170.71 | 174.39 | 174.86 | 169.81 | 169.78 | 168.23 | 169.53 | 169.56 |
| $H_2O$···$H_2O$ | $r$(O2-H1) | 0.9603 | 0.9586 | 0.9576 | 0.9554 | 0.9576 | 0.9572 | 0.9554 | 0.9559 | 0.9556 | 0.9601 | 0.9577 |
| | $r$(O2-H3) | 0.9671 | 0.9658 | 0.9649 | 0.9625 | 0.9654 | 0.9649 | 0.9626 | 0.9632 | 0.9629 | 0.9680 | 0.9648 |
| | $\theta$(H3-O2-H1) | 104.42 | 104.71 | 104.86 | 104.86 | 105.67 | 105.58 | 104.84 | 104.88 | 104.92 | 104.77 | 104.73 |
| | $r$(**H3-O4**) | 1.9600 | 1.9541 | 1.9503 | 1.9477 | 1.9472 | 1.9535 | 1.9507 | 1.9513 | 1.9487 | 1.9557 | 1.9618 |
| | $\theta$(**O4-H3-O2**) | 172.62 | 171.88 | 171.95 | 172.68 | 171.45 | 172.36 | 171.15 | 171.82 | 171.24 | 171.98 | 171.72 |
| | $r$(H5-O4) | 0.9618 | 0.9602 | 0.9593 | 0.9570 | 0.9587 | 0.9582 | 0.9570 | 0.9575 | 0.9572 | 0.9618 | 0.9593 |
| | $\theta$(**H5-O4-H3**) | 111.67 | 110.92 | 111.10 | 110.72 | 114.69 | 115.75 | 110.74 | 111.54 | 111.85 | 110.47 | 114.44 |
| | $\varphi$(**H5-O4-H3-O2**) | 58.32 | 58.01 | 58.17 | 57.83 | 60.23 | 60.89 | 57.89 | 58.46 | 58.67 | 57.78 | 58.36 |
| | $\theta$(H5-O4-H6) | 104.53 | 104.79 | 104.94 | 104.95 | 105.43 | 105.39 | 104.90 | 104.98 | 103.98 | 104.86 | 104.83 |
| $NH_3$···$H_2O$ | $r$(O1-H2) | 0.9601 | 0.9584 | 0.9574 | 0.9552 | 0.9574 | 0.9570 | 0.9552 | 0.9558 | 0.9555 | 0.9599 | 0.9576 |
| | $r$(O1-H3) | 0.9727 | 0.9714 | 0.9706 | 0.9680 | 0.9722 | 0.9717 | 0.9679 | 0.9688 | 0.9684 | 0.9742 | 0.9702 |
| | $\theta$(H3-O1-H2) | 104.65 | 104.93 | 105.09 | 105.07 | 106.12 | 106.03 | 105.05 | 105.16 | 105.14 | 104.99 | 104.96 |
| | $r$(**H3-N4**) | 1.9784 | 1.9733 | 1.9696 | 1.9731 | 1.9569 | 1.9604 | 1.9789 | 1.9738 | 1.9753 | 1.9707 | 1.9850 |
| | $\theta$(**N4-H3-O1**) | 170.87 | 170.53 | 170.45 | 170.77 | 166.01 | 166.23 | 169.86 | 169.91 | 169.84 | 170.81 | 169.98 |
| | $r$(H5-N4) | 1.0148 | 1.0133 | 1.0119 | 1.0107 | 1.0117 | 1.0112 | 1.0107 | 1.0110 | 1.0107 | 1.0142 | 1.0132 |
| | $\theta$(**H5-N4-H3**) | 103.53 | 102.96 | 102.76 | 102.36 | 101.02 | 101.18 | 102.22 | 102.40 | 102.47 | 103.12 | 102.63 |
| | $r$(H6-N4) | 1.0144 | 1.0128 | 1.0114 | 1.0102 | 1.0111 | 1.0107 | 1.0102 | 1.0105 | 1.0102 | 1.0137 | 1.0127 |
| | $\theta$(H6-N4-H5) | 106.54 | 106.72 | 106.90 | 106.88 | 107.26 | 107.21 | 106.89 | 106.91 | 106.90 | 106.88 | 106.70 |
| | $\varphi$(**H6-N4-H5-H3**) | 123.18 | 122.98 | 122.79 | 122.81 | 122.45 | 122.50 | 122.79 | 122.78 | 122.80 | 122.81 | 123.00 |

Table S6 Continued.

| | | CC/junVTZ | CC-F12/junTZ | CC-F12/junTZ+ MP2-CV(wCVTZ) | ChS | ChS+aug$\Delta\alpha$ | ChS+jun$\Delta\alpha$ | junChS | junCBS+CV-F12 | junChS-F12 | revDSD | Hobza |
|---|---|---|---|---|---|---|---|---|---|---|---|---|
| $CH_2O\cdots CH_2O$ | $r$(C1-H2) | 1.1015 | 1.1005 | 1.0990 | 1.0983 | 1.0981 | 1.0979 | 1.0985 | 1.099 | 1.099 | 1.1025 | 1.1011 |
| | $r$(C1-H3) | 1.1016 | 1.1008 | 1.0994 | 1.0989 | 1.0995 | 1.0992 | 1.0990 | 1.099 | 1.099 | 1.1023 | 1.1015 |
| | $\theta$(H3-C1-H2) | 117.52 | 117.64 | 117.66 | 117.62 | 117.91 | 117.87 | 117.60 | 117.60 | 117.58 | 117.42 | 117.60 |
| | $r$(O4-C1) | 1.2146 | 1.2117 | 1.2096 | 1.2068 | 1.2090 | 1.2087 | 1.2065 | 1.2065 | 1.2060 | 1.2104 | 1.2106 |
| | $\theta$(O4-C1-H3) | 121.12 | 121.07 | 121.06 | 121.10 | 120.96 | 120.97 | 121.10 | 121.09 | 121.11 | 121.41 | 121.31 |
| | $r$(**O5-H3**) | 2.4136 | 2.3949 | 2.3870 | 2.3776 | 2.3516 | 2.3787 | 2.3707 | 2.3839 | 2.3781 | 2.4143 | 2.3827 |
| | $\theta$(**O5-H3-C1**) | 121.62 | 121.35 | 121.43 | 121.41 | 120.98 | 121.07 | 121.29 | 121.33 | 121.25 | 120.86 | 121.55 |
| | $r$(C6-O5) | 1.2144 | 1.2116 | 1.2096 | 1.2070 | 1.2098 | 1.2093 | 1.2066 | 1.2064 | 1.2060 | 1.2106 | 1.2106 |
| | $\theta$(**C6-O5-H3**) | 98.30 | 98.37 | 98.46 | 98.38 | 98.41 | 98.53 | 98.37 | 98.41 | 98.50 | 98.09 | 98.34 |
| | $r$(H7-C6) | 1.1010 | 1.1000 | 1.0984 | 1.0977 | 1.0974 | 1.0972 | 1.0980 | 1.0983 | 1.0982 | 1.1018 | 1.1006 |
| | $\theta$(H7-C6-O5) | 121.79 | 121.77 | 121.75 | 121.78 | 121.59 | 121.56 | 121.82 | 121.80 | 121.80 | 121.88 | 121.79 |
| | $\varphi$(**H7-C6-O5-H3**) | 90.32 | 90.36 | 90.35 | 90.43 | 90.49 | 90.40 | 90.44 | 90.38 | 90.37 | 90.45 | 90.39 |
| $CH_4\cdots NH_3$ | $r$(C1-H2) | 1.0897 | 1.0885 | 1.0870 | 1.0857 | 1.0863 | 1.0856 | 1.0862 | 1.0865 | 1.0862 | 1.0898 | 1.0887 |
| | $r$(**H2-N3**) | 2.8166 | 2.8003 | 2.7948 | 2.8220 | 2.9307 | 2.9892 | 2.7713 | 2.7818 | 2.7751 | 2.7964 | 2.7933 |
| | $r$(C1-H4) | 1.0902 | 1.0888 | 1.0872 | 1.0861 | 1.0868 | 1.0862 | 1.0863 | 1.0866 | 1.0863 | 1.0901 | 1.0889 |
| | $\theta$(H4-C1-H2) | 109.72 | 109.72 | 109.72 | 109.70 | 109.63 | 109.62 | 109.71 | 109.71 | 109.71 | 109.72 | 109.71 |
| | $r$(H5-N3) | 1.0145 | 1.0129 | 1.0114 | 1.0103 | 1.0113 | 1.0108 | 1.0102 | 1.0105 | 1.0102 | 1.0138 | 1.0128 |
| | $\theta$(**H5-N3-H2**) | 112.44 | 112.27 | 112.07 | 112.08 | 111.69 | 111.73 | 112.06 | 112.05 | 112.06 | 112.11 | 112.26 |
| | $\theta$(H6-C1-H4) | 109.22 | 109.22 | 109.23 | 109.24 | 109.32 | 109.32 | 109.23 | 109.23 | 109.23 | 109.22 | 109.23 |
| | $\theta$(H5-N3-H8) | 106.34 | 106.54 | 106.75 | 106.74 | 107.16 | 107.12 | 106.77 | 106.77 | 106.76 | 106.71 | 106.54 |
| $CH_4\cdots HF$ | $r$(H2-F1) | 0.9223 | 0.9211 | 0.9206 | 0.9177 | 0.9220 | 0.9213 | 0.9173 | 0.9184 | 0.9179 | 0.9235 | 0.9193 |
| | $r$(**H2-C3**) | 2.3138 | 2.3022 | 2.2980 | 2.3191 | 2.3323 | 2.3444 | 2.3103 | 2.3077 | 2.3133 | 2.3079 | 2.3195 |
| | $r$(H4-C3) | 1.0886 | 1.0873 | 1.0857 | 1.0847 | 1.0856 | 1.0851 | 1.0850 | 1.0852 | 1.0849 | 1.0886 | 1.0873 |
| | $r$(H5-C3) | 1.0910 | 1.0897 | 1.0881 | 1.0870 | 1.0879 | 1.0873 | 1.0872 | 1.0876 | 1.0873 | 1.0909 | 1.0898 |
| | $\theta$(H5-C3-H4) | 108.74 | 108.72 | 108.70 | 108.74 | 108.66 | 108.63 | 108.75 | 108.74 | 108.76 | 108.70 | 108.76 |
| $NH_3\cdots NH_3$ | $r$(N1-H2) | 1.0159 | 1.0145 | 1.0131 | 1.0119 | 1.0127 | 1.0121 | 1.0120 | 1.0123 | 1.0120 | 1.0154 | 1.0145 |
| | $r$(**H2-N4**) | 2.1886 | 2.1760 | 2.1703 | 2.1627 | 2.2044 | 2.2250 | 2.1598 | 2.1612 | 2.1651 | 2.1802 | 2.1717 |
| | $\theta$(H3-H2-N1) | 98.14 | 98.01 | 98.08 | 98.40 | 98.47 | 98.46 | 98.29 | 98.30 | 98.16 | 98.15 | 98.17 |
| | $r$(H5-N4) | 1.0144 | 1.0128 | 1.0114 | 1.0102 | 1.0110 | 1.0105 | 1.0102 | 1.0105 | 1.0102 | 1.0137 | 1.0128 |
| | $\theta$(H5-N4-H3) | 106.70 | 106.88 | 107.09 | 107.09 | 107.73 | 107.64 | 107.15 | 107.13 | 107.14 | 107.05 | 106.89 |
| | $\varphi$(**H5-N4-H3-H2**) | 123.39 | 123.19 | 122.98 | 122.98 | 122.38 | 122.46 | 122.93 | 122.96 | 122.94 | 123.01 | 123.18 |

Table S6 Continued.

| | | CC/junVTZ | CC-F12/junTZ | CC-F12/junTZ+ MP2-CV(wCVTZ) | ChS | ChS+aug$\Delta\alpha$ | ChS+jun$\Delta\alpha$ | junChS | junCBS+CV-F12 | junChS-F12 | revDSD | Hobza |
|---|---|---|---|---|---|---|---|---|---|---|---|---|
| $CH_4 \cdots CH_4$ | $r$(C2-H1) | 1.0895 | 1.0882 | 1.0865 | 1.0856 | 1.0865 | 1.0897 | 1.0857 | 1.0860 | 1.0857 | 1.0894 | 1.0883 |
| | $r$**(C2-C3)** | 3.6953 | 3.6659 | 3.6605 | 3.6244 | 3.5438 | 3.6041 | 3.6231 | 3.6385 | 3.6373 | 3.6642 | 3.6380 |
| | $\theta$**(C3-C2-H1)** | 70.47 | 70.46 | 70.46 | 70.44 | 70.43 | 70.45 | 70.44 | 70.44 | 70.45 | 70.46 | 70.45 |
| | $r$(C3-H9) | 1.0895 | 1.0882 | 1.0866 | 1.0855 | 1.0863 | 1.0895 | 1.0857 | 1.0860 | 1.0857 | 1.0894 | 1.0882 |
| $C_2H_4 \cdots C_2H_4$ | $r$(C1-C6) | 1.3383 | 1.3350 | 1.3318 | 1.3302 | 1.3312 | 1.3312 | 1.3302 | 1.3335 | 1.3299 | 1.3319 | 1.3346 |
| | $r$**(X2-X3)** | 3.8497 | 3.8347 | 3.8232 | 3.7915 | 3.7102 | 3.7795 | 3.7816 | 3.8142 | 3.7994 | 3.8216 | 3.8116 |
| | $r$(C4-C5) | 1.3381 | 1.3348 | 1.3316 | 1.3301 | 1.3313 | 1.3313 | 1.3298 | 1.3333 | 1.3295 | 1.3316 | 1.3342 |
| | $r$(C4-H7) | 1.0836 | 1.0826 | 1.0812 | 1.0806 | 1.0813 | 1.0809 | 1.0807 | 1.0824 | 1.0807 | 1.0837 | 1.0832 |
| | $\theta$(H7-C4-C5) | 121.07 | 121.03 | 121.01 | 121.01 | 120.93 | 121.03 | 121.01 | 121.01 | 121.00 | 121.06 | 121.03 |
| | $r$(H8-C4) | 1.0837 | 1.0826 | 1.0811 | 1.0806 | 1.0812 | 1.0808 | 1.0806 | 1.0823 | 1.0806 | 1.0837 | 1.0832 |
| | $\theta$(H8-C4-C5) | 121.53 | 121.52 | 121.52 | 121.54 | 121.56 | 121.53 | 121.54 | 121.52 | 121.53 | 121.60 | 121.52 |
| | $\theta$**(C1-C6-C5)** | 90.00 | 89.93 | 90.00 | 90.00 | 90.00 | 90.00 | 90.00 | 90.00 | 89.92 | 90.00 | 90.00 |
| | $r$(H12-C1) | 1.0837 | 1.0826 | 1.0811 | 1.0805 | 1.0812 | 1.0808 | 1.0806 | 1.0823 | 1.0806 | 1.0837 | 1.0831 |
| | $\theta$(H12-C1-C6) | 121.42 | 121.40 | 121.40 | 121.41 | 121.39 | 121.41 | 121.42 | 121.40 | 121.40 | 121.46 | 121.41 |
| | $\varphi$**(H12-C1-C4-C5)** | -121.42 | -121.40 | -121.40 | -121.41 | -121.39 | -121.41 | -121.42 | -121.40 | -121.40 | -121.46 | -121.41 |
| $C_2H_4 \cdots CH_2O$ | $r(C_1{=}O_2)$ | 1.2126 | 1.2096 | 1.2075 | 1.2047 | 1.2069 | 1.2053 | 1.2044 | 1.2044 | 1.2039 | 1.2084 | 1.2084 |
| | $r$(H3-C1) | 1.1031 | 1.1022 | 1.1006 | 1.1000 | 1.0998 | 1.1024 | 1.1002 | 1.1005 | 1.1004 | 1.1043 | 1.1028 |
| | $\theta$(H3-C1-O2) | 121.45 | 121.42 | 121.40 | 121.44 | 121.28 | 121.29 | 121.44 | 121.45 | 121.73 | 121.52 | 121.43 |
| | $r$(H4-C1) | 1.1022 | 1.1014 | 1.0999 | 1.0994 | 1.0995 | 1.1021 | 1.0998 | 1.0997 | 1.1106 | 1.1032 | 1.1021 |
| | $\theta$(H4-C1-O2) | 121.50 | 121.46 | 121.44 | 121.47 | 121.30 | 121.39 | 121.48 | 121.49 | 121.79 | 121.57 | 121.48 |
| | $r$**(H4-C5)** | 2.8807 | 2.8650 | 2.8572 | 2.8344 | 2.7848 | 2.8293 | 2.8472 | 2.8488 | 2.8748 | 2.8706 | 2.8607 |
| | $\theta$**(C5-H4-C1)** | 114.22 | 114.08 | 114.11 | 115.21 | 116.54 | 117.54 | 114.38 | 114.13 | 109.28 | 114.10 | 114.19 |
| | $r$(C5-C6) | 1.3388 | 1.3355 | 1.3323 | 1.3307 | 1.3319 | 1.3366 | 1.3306 | 1.3303 | 1.3435 | 1.3324 | 1.3350 |
| | $\theta$**(C6-C5-C1)** | 94.11 | 94.12 | 93.56 | 94.63 | 91.20 | 96.75 | 94.34 | 93.12 | 93.24 | 109.76 | 108.45 |
| | $r$(H7-C5) | 1.0833 | 1.0822 | 1.0808 | 1.0801 | 1.0808 | 1.0833 | 1.0805 | 1.0803 | 1.0909 | 1.0833 | 1.0827 |
| | $\theta$(H7-C5-C6) | 121.72 | 121.72 | 121.72 | 121.73 | 121.69 | 121.83 | 121.72 | 121.71 | 121.74 | 121.76 | 121.71 |
| | $\varphi$**(H7-C5-C6-H4)** | 89.78 | 89.75 | 89.74 | 89.82 | 89.78 | 89.83 | 89.73 | 89.72 | 89.73 | 89.76 | 89.72 |
| | $r$(H9-C6) | 1.0838 | 1.0827 | 1.0812 | 1.0806 | 1.0812 | 1.0836 | 1.0809 | 1.0807 | 1.0917 | 1.0838 | 1.0833 |
| | $\theta$(H9-C6-C5) | 121.48 | 121.46 | 121.46 | 121.47 | 121.46 | 121.59 | 121.46 | 121.46 | 121.48 | 121.52 | 121.47 |
| | $\varphi$**(H9-C6-C5-H4)** | -90.16 | -90.17 | -90.18 | -90.17 | -90.21 | -90.19 | -90.18 | -90.20 | -90.18 | -90.17 | -90.18 |

Table S6 Continued.

| | | CC/junVTZ | CC-F12/junTZ | CC-F12/junTZ+ MP2-CV(wCVTZ) | ChS | ChS+aug$\Delta\alpha$ | ChS+jun$\Delta\alpha$ | junChS | junCBS+CV-F12 | junChS-F12 | revDSD | Hobza |
|---|---|---|---|---|---|---|---|---|---|---|---|---|
| $C_2H_4 \cdots H_2O$ | $r$(H1-O2) | 0.9609 | 0.9592 | 0.9583 | 0.9562 | 0.9582 | 0.9577 | 0.9561 | 0.9566 | 0.9563 | 0.9608 | 0.9584 |
| | $r$(H3-O2) | 0.9641 | 0.9626 | 0.9617 | 0.9594 | 0.9625 | 0.9621 | 0.9593 | 0.9599 | 0.9595 | 0.9646 | 0.9615 |
| | $\theta$(H3-O2-H1) | 104.25 | 104.53 | 104.69 | 104.68 | 105.72 | 105.63 | 104.68 | 104.76 | 104.74 | 104.63 | 104.64 |
| | $r$(**H3-X4**) | 2.4206 | 2.4168 | 2.4105 | 2.4199 | 2.4157 | 2.4272 | 2.4252 | 2.4242 | 2.4283 | 2.4006 | 2.4224 |
| | $\theta$(**O2-H3-X4**) | 173.41 | 173.41 | 173.27 | 177.41 | 163.64 | 163.99 | 170.75 | 172.87 | 172.72 | 166.39 | 161.14 |
| | $r$(C5-C6) | 1.3397 | 1.3364 | 1.3332 | 1.3317 | 1.3327 | 1.3328 | 1.3316 | 1.3317 | 1.3313 | 1.3336 | 1.3361 |
| | $r$(C5-H8) | 1.0836 | 1.0826 | 1.0811 | 1.0804 | 1.0811 | 1.0807 | 1.0805 | 1.0808 | 1.0805 | 1.0837 | 1.0832 |
| | $\theta$(H8-C5-C6) | 121.45 | 121.44 | 121.43 | 121.43 | 121.39 | 121.41 | 121.45 | 121.44 | 121.44 | 121.49 | 121.42 |
| | $r$(H7-C5) | 1.0836 | 1.0826 | 1.0811 | 1.0804 | 1.0810 | 1.0807 | 1.0805 | 1.0808 | 1.0805 | 1.0837 | 1.0831 |
| | $\theta$(H7-C5-C6) | 121.45 | 121.44 | 121.43 | 121.45 | 121.44 | 121.43 | 121.46 | 121.44 | 121.44 | 121.47 | 121.41 |
| | $\varphi$(**C5-H3-O2-H1**) | -112.51 | -112.53 | -112.95 | -112.99 | -160.01 | -159.49 | -117.80 | -114.32 | -114.81 | -130.26 | -139.53 |
| | $\varphi$(**H8-C5-X4-H3**) | -90.10 | -90.10 | -90.11 | -85.09 | -79.53 | -80.52 | -87.57 | -90.11 | -90.12 | -77.76 | -72.92 |
| $C_2H_4 \cdots NH_3$ | $r$(C1-C2) | 1.3388 | 1.3356 | 1.3324 | 1.3308 | 1.3320 | 1.3366 | 1.3307 | 1.3308 | 1.3304 | 1.3325 | 1.3351 |
| | $r$(**C2-H3**) | 2.6878 | 2.6778 | 2.6698 | 2.6953 | 2.6880 | 2.7529 | 2.6616 | 2.6661 | 2.6694 | 2.6706 | 2.6835 |
| | $\theta$(**C1-C2-H3**) | 88.55 | 88.88 | 88.28 | 82.88 | 73.54 | 77.77 | 87.38 | 86.99 | 86.73 | 87.02 | 86.93 |
| | $r$(H3-N4) | 1.0150 | 1.0136 | 1.0122 | 1.0111 | 1.0122 | 1.0137 | 1.0111 | 1.0112 | 1.0110 | 1.0146 | 1.0135 |
| | $\theta$(**C2-H3-N4**) | 146.07 | 145.67 | 146.51 | 157.89 | 173.55 | 170.12 | 148.10 | 148.23 | 148.46 | 147.48 | 147.84 |
| | $r$(N4-H5) | 1.0145 | 1.0129 | 1.0114 | 1.0101 | 1.0107 | 1.0129 | 1.0102 | 1.0104 | 1.0102 | 1.0138 | 1.0126 |
| | $\theta$(H3-N4-H5) | 106.53 | 106.73 | 106.94 | 106.89 | 107.74 | 107.28 | 107.00 | 106.99 | 106.99 | 106.90 | 104.75 |
| | $\varphi$(**C2-H3-N4-H5**) | 123.42 | 123.23 | 123.01 | 123.05 | 122.24 | 122.68 | 122.95 | 122.96 | 122.96 | 123.05 | 123.22 |
| | $r$(C2-H7) | 1.0835 | 1.0824 | 1.0810 | 1.0803 | 1.0811 | 1.0835 | 1.0804 | 1.0806 | 1.0804 | 1.0835 | 1.0828 |
| | $\theta$(C1-C2-H7) | 121.53 | 121.52 | 121.51 | 121.48 | 121.38 | 121.52 | 121.53 | 121.50 | 121.50 | 121.57 | 121.52 |
| | $\varphi$(**H7-C2-C1-H3**) | 89.87 | 89.85 | 89.84 | 89.91 | 90.03 | 90.02 | 89.85 | 89.84 | 89.85 | 89.87 | 89.85 |
| | $r$(C1-H9) | 1.0837 | 1.0826 | 1.0811 | 1.0804 | 1.0810 | 1.0835 | 1.0805 | 1.0808 | 1.0806 | 1.0837 | 1.0830 |
| | $\theta$(C2-C1-H9) | 121.46 | 121.44 | 121.44 | 121.45 | 121.425 | 121.55 | 121.46 | 121.44 | 121.44 | 121.50 | 121.45 |
| | $\varphi$(**H9-C1-C2-H3**) | -90.12 | -90.13 | -90.14 | -90.16 | -90.17 | -90.16 | -90.15 | -90.14 | -90.15 | -90.13 | -90.14 |

Table S6 Continued.

| | | CC/junVTZ | CC-F12/junTZ | CC-F12/junTZ+ MP2-CV(wCVTZ) | ChS | ChS+aug$\Delta\alpha$ | ChS+jun$\Delta\alpha$ | junChS | junCBS+CV-F12 | junChS-F12 | revDSD | Hobza |
|---|---|---|---|---|---|---|---|---|---|---|---|---|
| $H_2O\cdots CH_4$ | $r$(C2-H3) | 1.0888 | 1.0880 | 1.0864 | 1.0857 | 1.0869 | 1.0862 | 1.0852 | 1.0859 | 1.0857 | 1.0893 | 1.0880 |
| | $r$(**H3-O4**) | 2.6659 | 2.6270 | 2.6232 | 2.8410 | 2.7831 | 2.8169 | 2.6434 | 2.6238 | 2.6229 | 2.6445 | 2.6279 |
| | $r$(H1-C2) | 1.0898 | 1.0886 | 1.0870 | 1.0863 | 1.0869 | 1.0863 | 1.0860 | 1.0864 | 1.0861 | 1.0900 | 1.0887 |
| | $r$(H7-C2) | 1.0892 | 1.0887 | 1.0870 | 1.0856 | 1.0867 | 1.0862 | 1.0854 | 1.0865 | 1.0861 | 1.0899 | 1.0887 |
| | $r$(H5-O4) | 0.9601 | 0.9596 | 0.9586 | 0.9565 | 0.9582 | 0.9577 | 0.9553 | 0.9569 | 0.9566 | 0.9612 | 0.9583 |
| | $\theta$(**O4-H3-C2**) | 161.98 | 179.96 | 179.87 | 141.28 | 157.40 | 158.17 | 161.25 | 179.74 | 179.60 | 179.41 | 179.09 |
| | $\theta$(H1-C2-H3) | 109.94 | 109.67 | 109.68 | 109.73 | 109.49 | 109.44 | 109.93 | 109.66 | 109.67 | 109.70 | 109.65 |
| | $\theta$(H7-C2-H3) | 109.55 | 109.29 | 109.66 | 109.58 | 109.69 | 109.70 | 109.55 | 109.67 | 109.30 | 109.66 | 109.68 |
| | $\theta$(**H5-O4-H3**) | 80.35 | 127.77 | 127.30 | 77.91 | 118.12 | 125.06 | 80.26 | 127.88 | 127.30 | 123.52 | 127.69 |
| | $\varphi$(**H5-O4-H3-C2**) | 52.82 | 89.94 | 82.77 | 53.89 | 68.17 | 91.56 | 51.26 | 89.96 | 82.74 | 71.54 | 87.36 |
| | $\varphi$(**H8-C2-H3-O4**) | -120.09 | -120.02 | -120.03 | -120.01 | -119.94 | -119.93 | -120.08 | -120.02 | -120.03 | -120.03 | -120.02 |

Table S7: ChS, junChS, and junChS-F12 models: CBS and CV contributions for the A14 complexes. The inter-molecular parameters are highlighted in bold.

| | | $\Delta R$(CBS) | | | $\Delta R$(CV) |
|---|---|---|---|---|---|
| | | ChS | junChS | junChS-F12 | |
| HCN···HCN | $r$(H1-C2) | -0.0009 | -0.0021 | -0.0006 | -0.0012 |
| | $r$(C2-N3) | -0.0055 | -0.0055 | -0.0024 | -0.0025 |
| | $r$(N3-H4) | 0.0035 | 0.0021 | 0.0048 | -0.0024 |
| | $r$(**H4-C5**) | 0.0002 | -0.0014 | -0.0001 | -0.0012 |
| | $r$(C5-N6) | -0.0055 | -0.0057 | -0.0025 | -0.0024 |
| HF···HF | $r$(H1-F2) | -0.0022 | -0.0046 | -0.0027 | -0.0005 |
| | $r$(**F2-H3**) | 0.0146 | -0.0110 | -0.0032 | -0.0018 |
| | $r$(H3-F4) | -0.0012 | -0.0043 | 0.0462 | -0.0005 |
| | $\theta$(**H3-F2-F1**) | 5.53 | -0.60 | -0.003 | 0.21 |
| | $\theta$(**F4-H3-F2**) | 3.88 | -0.93 | -1.44 | 0.11 |
| $H_2O$···$H_2O$ | $r$(O2-H1) | -0.0024 | -0.0042 | -0.0020 | -0.0008 |
| | $r$(O2-H3) | -0.0016 | -0.0038 | -0.0020 | -0.0008 |
| | $\theta$(H3-O2-H1) | 1.04 | 0.31 | 0.05 | 0.11 |
| | $r$(**H3-O4**) | -0.0055 | -0.0066 | -0.0016 | -0.0027 |
| | $\theta$(**O4-H3-O2**) | -0.55 | -1.59 | -0.71 | 0.12 |
| | $r$(H5-O4) | -0.0029 | -0.0038 | -0.0021 | -0.0008 |
| | $\theta$(**H5-O4-H3**) | 3.23 | -1.12 | 0.74 | 0.21 |
| | $\varphi$(**H5-O4-H3-O2**) | 2.01 | -0.59 | 0.50 | 0.16 |
| | $\theta$(H5-O4-H6) | 0.73 | 0.26 | 0.04 | 0.12 |

Table: S7 Continued.

| | | ΔR(CBS) | | | ΔR(CV) |
|---|---|---|---|---|---|
| | | ChS | junChS | junChS-F12 | |
| $NH_3 \cdots H_2O$ | $r$(O1-H2) | -0.0026 | -0.0040 | -0.0020 | -0.0008 |
| | $r$(O1-H3) | -0.0007 | -0.0042 | -0.0023 | -0.0007 |
| | $\theta$(H3-O1-H2) | 1.23 | 0.28 | 0.05 | 0.12 |
| | $r$**(H3-N4)** | -0.0154 | 0.0028 | 0.0057 | -0.0025 |
| | $\theta$**(N4-H3-O1)** | -4.38 | -1.00 | -0.61 | -0.02 |
| | $r$(H5-N4) | -0.0024 | -0.0029 | -0.0012 | -0.0012 |
| | $\theta$**(H5-N4-H3)** | -2.08 | -1.16 | -0.29 | -0.14 |
| | $r$(H6-N4) | -0.0024 | -0.0029 | -0.0012 | -0.0012 |
| | $\theta$(H6-N4-H5) | 0.55 | 0.21 | -0.001 | 0.14 |
| | $\varphi$**(H6-N4-H5-H3)** | -0.54 | -0.24 | 0.001 | -0.15 |
| $CH_2O \cdots CH_2O$ | $r$(C1-H2) | -0.0022 | -0.0017 | -0.0001 | -0.0013 |
| | $r$(C1-H3) | -0.0010 | -0.0012 | -0.0001 | -0.0013 |
| | $\theta$(H3-C1-H2) | 0.35 | 0.07 | -0.04 | 0.001 |
| | $r$(O4-C1) | -0.0040 | -0.0061 | -0.0015 | -0.0020 |
| | $\theta$(O4-C1-H3) | -0.17 | -0.03 | 0.02 | 0.003 |
| | $r$**(O5-H3)** | -0.0370 | -0.0396 | -0.0038 | -0.0032 |
| | $\theta$**(O5-H3-C1)** | -0.57 | -0.36 | -0.07 | 0.03 |
| | $r$(C6-O5) | -0.0035 | -0.0059 | -0.0015 | -0.0020 |
| | $\theta$**(C6-O5-H3)** | 0.16 | 0.03 | 0.02 | 0.04 |
| | $r$(H7-C6) | -0.0024 | -0.0016 | -0.0001 | -0.0013 |
| | $\theta$(H7-C6-O5) | -0.21 | 0.05 | 0.02 | -0.002 |
| | $\varphi$**(H7-C6-O5-H3)** | 0.10 | 0.12 | 0.01 | -0.01 |

Table: S7 Continued.

| | | ΔR(CBS) | | | ΔR(CV) |
|---|---|---|---|---|---|
| | | ChS | junChS | junChS-F12 | |
| $CH_4\cdots NH_3$ | $r$(C1-H2) | -0.0024 | -0.0021 | -0.0008 | -0.0014 |
| | $r$**(H2-N3)** | 0.1489 | -0.0426 | -0.0198 | -0.0027 |
| | $r$(C1-H4) | -0.0024 | -0.0024 | -0.0009 | -0.0014 |
| | $\theta$(H4-C1-H2) | -0.10 | -0.02 | -0.002 | -0.004 |
| | $r$(H5-N3) | -0.0026 | -0.0031 | -0.0012 | -0.0012 |
| | $\theta$**(H5-N3-H2)** | -0.55 | -0.24 | -0.01 | -0.15 |
| | $\theta$(H6-C1-H4) | 0.10 | 0.02 | 0.002 | 0.004 |
| | $\theta$(H5-N3-H8) | 0.61 | 0.24 | 0.01 | 0.17 |
| $CH_4\cdots HF$ | $r$(H2-F1) | -0.0007 | -0.0045 | -0.0027 | -0.0005 |
| | $r$**(H2-C3)** | 0.0296 | 0.0007 | 0.0153 | -0.0041 |
| | $r$(H4-C3) | -0.0019 | -0.0022 | -0.0008 | -0.0014 |
| | $r$(H5-C3) | -0.0021 | -0.0022 | -0.0008 | -0.0015 |
| | $\theta$(H5-C3-H4) | -0.10 | 0.03 | 0.05 | -0.01 |
| $NH_3\cdots NH_3$ | $r$(N1-H2) | -0.0025 | -0.0027 | -0.0012 | -0.0012 |
| | $r$**(H2-N4)** | 0.0373 | -0.0251 | -0.0052 | -0.0038 |
| | $\theta$(H3-H2-N1) | 0.09 | 0.06 | 0.07 | 0.10 |
| | $r$(H5-N4) | -0.0027 | -0.003 | -0.0012 | -0.0012 |
| | $\theta$(H5-N4-H3) | 0.76 | 0.29 | 0.05 | 0.16 |
| | $\varphi$**(H5-N4-H3-H2)** | -0.73 | -0.29 | -0.04 | -0.16 |

Table: S7 Continued.

| | | ΔR(CBS) | | | ΔR(CV) |
|---|---|---|---|---|---|
| | | ChS | junChS | junChS-F12 | |
| $CH_4 \cdots CH_4$ | $r$(C2-H1) | -0.0020 | -0.0024 | -0.0008 | -0.0014 |
| | $r$**(C2-C3)** | -0.0746 | -0.0696 | -0.0232 | -0.0026 |
| | $\theta$**(C3-C2-H1)** | -0.01 | -0.03 | -0.02 | -0.001 |
| | $r$(C3-H9) | -0.0022 | -0.0024 | -0.0009 | -0.0014 |
| $C_2H_4 \cdots C_2H_4$ | $r$(C1-C6) | -0.0045 | -0.0053 | -0.0019 | -0.0028 |
| | $r$**(X2-X3)** | -0.0685 | -0.0611 | -0.0239 | -0.0070 |
| | $r$(C4-C5) | -0.0042 | -0.0055 | -0.0021 | -0.0028 |
| | $r$(C4-H7) | -0.0014 | -0.0016 | -0.0004 | -0.0013 |
| | $\theta$(H7-C4-C5) | -0.04 | -0.06 | -0.01 | 0.003 |
| | $r$(H8-C4) | -0.0016 | -0.0018 | -0.0005 | -0.0013 |
| | $\theta$(H8-C4-C5) | -0.01 | 0.001 | 0.01 | 0.01 |
| | $\theta$**(C1-C6-C5)** | 0.001 | 0.001 | -0.01 | 0.00 |
| | $r$(H12-C1) | -0.0016 | -0.0018 | -0.0005 | -0.0013 |
| | $\theta$(H12-C1-C6) | 0.02 | 0.01 | -0.002 | -0.01 |
| | $\varphi$**(H12-C1-C4-C5)** | -0.02 | -0.01 | 0.002 | 0.01 |

Table: S7 Continued.

| | | ΔR(CBS) | | | ΔR(CV) |
|---|---|---|---|---|---|
| | | ChS | junChS | junChS-F12 | |
| | $r(C_1{=}O_2)$ | -0.0042 | -0.0063 | -0.0037 | -0.0020 |
| | $r$(H3-C1) | -0.0021 | -0.0016 | -0.0003 | -0.0013 |
| | $\theta$(H3-C1-O2) | -0.19 | 0.003 | 0.05 | -0.002 |
| | $r$(H4-C1) | -0.0016 | -0.0014 | -0.0002 | -0.0013 |
| | $\theta$(H4-C1-O2) | -0.16 | 0.001 | 0.05 | -0.01 |
| | $r$**(H4-C5)** | -0.0511 | -0.0375 | -0.0085 | -0.0043 |
| | $\theta$**(C5-H4-C1)** | 2.23 | -0.24 | 0.01 | 0.03 |
| $C_2H_4 \cdots CH_2O$ | $r$(C5-C6) | -0.0042 | -0.0053 | -0.002 | -0.0028 |
| | $\theta$**(C6-C5-C1)** | -1.95 | -1.29 | -0.44 | -0.18 |
| | $r$(H7-C5) | -0.0015 | -0.0018 | -0.0005 | -0.0013 |
| | $\theta$(H7-C5-C6) | -0.04 | -0.01 | -0.01 | 0.01 |
| | $\varphi$**(H7-C5-C6-H4)** | 0.02 | -0.03 | -0.02 | -0.001 |
| | $r$(H9-C6) | -0.0016 | -0.0018 | -0.0005 | -0.0013 |
| | $\theta$(H9-C6-C5) | -0.02 | -0.01 | 0.002 | 0.01 |
| | $\varphi$**(H9-C6-C5-H4)** | -0.02 | -0.02 | -0.01 | -0.004 |

Table: S7 Continued.

| | | $\Delta R$(CBS) | | | $\Delta R$(CV) |
|---|---|---|---|---|---|
| | | ChS | junChS | junChS-F12 | |
| $C_2H_4 \cdots H_2O$ | $r$(H1-O2) | -0.0025 | -0.004 | -0.0020 | -0.0008 |
| | $r$(H3-O2) | -0.0013 | -0.004 | -0.0022 | -0.0008 |
| | $\theta$(H3-O2-H1) | 1.19 | 0.31 | 0.05 | 0.12 |
| | $r$**(H3-X4)** | 0.0049 | 0.0084 | 0.0179 | -0.0038 |
| | $\theta$**(O2-H3-X4)** | -9.22 | -2.71 | -0.56 | 0.05 |
| | $r$(C5-C6) | -0.0042 | -0.0053 | -0.0019 | -0.0028 |
| | $r$(C5-H8) | -0.0016 | -0.0018 | -0.0006 | -0.0013 |
| | $\theta$(H8-C5-C6) | -0.03 | -0.02 | 0.003 | 0.01 |
| | $r$(H7-C5) | -0.0016 | -0.0018 | -0.0006 | -0.0013 |
| | $\theta$(H7-C5-C6) | -0.02 | -0.004 | 0.003 | 0.01 |
| | $\varphi$**(C5-H3-O2-H1)** | -45.31 | -5.12 | -1.76 | 0.17 |
| | $\varphi$**(H8-C5-X4-H3)** | 4.99 | 2.48 | -0.01 | 0.05 |

Table: S7 Continued.

| | | ΔR(CBS) | | | ΔR(CV) |
|---|---|---|---|---|---|
| | | ChS | junChS | junChS-F12 | |
| $C_2H_4 \cdots NH_3$ | $r$(C1-C2) | -0.0042 | -0.0053 | -0.0019 | -0.0028 |
| | $r$**(C2-H3)** | 0.0164 | -0.0211 | -0.0004 | -0.0052 |
| | $\theta$**(C1-C2-H3)** | -14.60 | -0.74 | -1.55 | -0.43 |
| | $r$(H3-N4) | -0.0023 | -0.0028 | -0.0011 | -0.0012 |
| | $\theta$**(C2-H3-N4)** | 27.28 | 1.28 | 1.95 | 0.75 |
| | $r$(N4-H5) | -0.0029 | -0.003 | -0.0012 | -0.0012 |
| | $\theta$(H3-N4-H5) | 0.89 | 0.30 | 0.05 | 0.17 |
| | $\varphi$**(C2-H3-N4-H5)** | -0.86 | -0.30 | -0.05 | -0.17 |
| | $r$(C2-H7) | -0.0014 | -0.0018 | -0.0005 | -0.0013 |
| | $\theta$(C1-C2-H7) | -0.16 | -0.01 | -0.01 | 0.01 |
| | $\varphi$**(H7-C2-C1-H3)** | 0.18 | -0.01 | 0.003 | 0.002 |
| | $r$(C1-H9) | -0.0017 | -0.0018 | -0.0005 | -0.0013 |
| | $\theta$(C2-C1-H9) | -0.03 | -0.01 | 0.004 | 0.01 |
| | $\varphi$**(H9-C1-C2-H3)** | -0.03 | -0.02 | -0.02 | -0.003 |

Table: S7 Continued.

| | | $\Delta R$(CBS) | | | $\Delta R$(CV) |
|---|---|---|---|---|---|
| | | ChS | junChS | junChS-F12 | |
| | $r$(C2-H3) | -0.0017 | -0.0022 | -0.0008 | -0.0014 |
| | $r$(**H3-O4**) | 0.1777 | -0.0199 | -0.0003 | -0.0026 |
| | $r$(H1-C2) | -0.0021 | -0.0024 | -0.0009 | -0.0014 |
| | $r$(H7-C2) | -0.0022 | -0.0024 | -0.0009 | -0.0014 |
| | $r$(H5-O4) | -0.0028 | -0.004 | -0.0020 | -0.0008 |
| $H_2O\cdots CH_4$ | $\theta$(**O4-H3-C2**) | -20.56 | -0.59 | -0.28 | -0.14 |
| | $\theta$(H1-C2-H3) | -0.21 | -0.02 | -0.01 | 0.002 |
| | $\theta$(H7-C2-H3) | 0.03 | -0.003 | -0.004 | -0.002 |
| | $\theta$(**H5-O4-H3**) | -2.49 | -0.14 | -0.003 | 0.05 |
| | $\varphi$(**H5-O4-H3-C2**) | 1.02 | -1.61 | 0.003 | 0.05 |
| | $\varphi$(**H8-C2-H3-O4**) | 0.08 | 0.004 | 0.004 | -0.002 |

Table S8: Comparison of CP and NCP corrected geometries for some paradigmatic cases at the augF12CBS+CV and augF12CBS+CV-F12 levels.

| | | augF12CBS+CV[a] | augF12CBS+CV-F12[b] |
|---|---|---|---|
| | | NCP | NCP |
| $H_2O\cdots H_2S$ | $r$(O1-H2) | 0.9641 | 0.9623 |
| | $r$(O1-H3) | 0.9598 | 0.9581 |
| | $\theta$(H2-O1-H3) | 104.52 | 104.69 |
| | $r$(H3$\cdots$S4) | 3.4639 | 3.4783 |
| | $\theta$(O1-H3-S4) | 116.65 | 116.61 |
| | $r$(H5/H6-S4) | 1.3395 | 1.3379 |
| | $\theta$(H5-S4-H3) | 83.02 | 83.85 |
| | $\varphi$(H5-S4-H3-O1) | 133.49 | 133.48 |
| | $\varphi$(H6-S4-H3-O1) | -133.49 | -133.48 |
| | $\theta$(H5-S4-H6) | 92.15 | 92.35 |
| $H_2O\cdots H_2O$ | $r$(O2-H1) | 0.9592 | 0.9574 |
| | $r$(O2-H3) | 0.9664 | 0.9647 |
| | $\theta$(H3-O2-H1) | 104.67 | 104.83 |
| | $r$(H3$\cdots$O4) | 1.9442 | 1.9494 |
| | $\theta$(O4-H3-O2) | 171.54 | 171.72 |
| | $r$(H5/H6-O4) | 0.9607 | 0.9590 |
| | $\theta$(H5-O4-H3) | 111.01 | 111.51 |
| | $\varphi$(H5-O4-H3-O2) | 58.04 | 58.43 |
| | $\varphi$(H6-O4-H3-O2) | -58.04 | -58.43 |
| | $\theta$(H5-O4-H6) | 104.75 | 104.92 |
| $CH_4\cdots CH_4$ | $r$(C2-H1) | 1.0889 | 1.0870 |
| | $r$(C2$\cdots$C3) | 3.6294 | 3.6470 |
| | $\theta$(C3-C2-H1) | 70.44 | 70.45 |
| | $r$(C3-H9) | 1.0889 | 1.0870 |
| HCN$\cdots$HCN | $r$(H1-C2) | 1.0679 | 1.0664 |
| | $r$(C2-N3) | 1.1545 | 1.1522 |
| | $r$(N3$\cdots$H4) | 2.2108 | 2.2120 |
| | $r$(H4-C5) | 1.0737 | 1.0723 |
| | $r$(C5-N6) | 1.1567 | 1.1544 |

[a] Conventional CBS+CV scheme using the aug-cc-pV$n$Z-F12 basis sets.
[b] CBS+CV-F12 scheme using the aug-cc-pV$n$Z-F12 basis sets.
